# Supplementary material for: Unified Human-Scene Interaction via Prompted Chain-of-Contacts
Source: arXiv:2309.07918 source file (2024-11-05)
Supplement: Supplementary file 1 [file supp.tex]

\documentclass{article} % For LaTeX2e
\usepackage{iclr2024_conference,times}

% Optional math commands from https://github.com/goodfeli/dlbook_notation.
\input{math_commands.tex}

\usepackage{booktabs} % /toprule
\usepackage{multirow}
\usepackage{makecell}
\usepackage{hyperref}
\usepackage{url}
\usepackage{graphicx} % for scalebox
\usepackage{bbding} % for \XSolid

\usepackage{xspace}

\usepackage{amsmath}
\usepackage{diagbox}
\usepackage{wrapfig}

\usepackage{longtable}
% \usepackage[section]{placeins} % avoid table floating
% \usepackage[misc]{ifsym} % \Letter

% \title{Unified Physical Human-Scene Interaction with Large Language Models in the Loop}
% \title{Unified Physical Human-Scene Interaction with Large Language Models as Planners}
% \usepackage{authblk}
% \title{
% \begin{minipage}{.10\textwidth}
% \includegraphics[width=\linewidth]{figures/unihsi_icon.png} 
% \end{minipage}%
% \begin{minipage}{.90\textwidth}
% \begin{center}
% Interact As I Say: \\
% Unified Human-Scene Interaction \\
% as Chain of Contacts
% \end{center}
% \end{minipage}
% }

\title{
Unified Human-Scene Interaction via \\ Prompted Chain-of-Contacts
}

% Authors must not appear in the submitted version. They should be hidden
% as long as the \iclrfinalcopy macro remains commented out below.
% Non-anonymous submissions will be rejected without review.

% \author{Zeqi Xiao$^{1,2}$\quad
% Tai Wang$^{1,}$\quad
% Jingbo Wang$^{1}$\quad
% Jinkun Cao$^{3}$\quad
% Wenwei Zhang$^{1}$\quad
% Bo Dai$^{1}$\quad
% Dahua Lin$^{1}$\quad
% Jiangmiao Pang$^{1\textrm{\Letter}}$\\
% $^1$Shanghai AI Laboratory\quad
% $^2$S-Lab, NTU\quad
% $^3$CMU\\
% {\tt\small \{zeqixiao1,pangjiangmiao\}@gmail.com, \{wenwei001,ccloy\}@ntu.edu.sg, \{wt019,dhlin\}@ie.cuhk.edu.hk}
% }

\author{Antiquus S.~Hippocampus, Natalia Cerebro \& Amelie P. Amygdale \thanks{ Use footnote for providing further information
about author (webpage, alternative address)---\emph{not} for acknowledging
funding agencies.  Funding acknowledgements go at the end of the paper.} \\
Department of Computer Science\\
Cranberry-Lemon University\\
Pittsburgh, PA 15213, USA \\
\texttt{\{hippo,brain,jen\}@cs.cranberry-lemon.edu} \\
\And
Ji Q. Ren \& Yevgeny LeNet \\
Department of Computational Neuroscience \\
University of the Witwatersrand \\
Joburg, South Africa \\
\texttt{\{robot,net\}@wits.ac.za} \\
\AND
Coauthor \\
Affiliation \\
Address \\
\texttt{email}
}

% \author{Ze S.~Hippocampus, Natalia Cerebro \& Amelie P. Amygdale \thanks{ Use footnote for providing further information
% about author (webpage, alternative address)---\emph{not} for acknowledging
% funding agencies.  Funding acknowledgments go at the end of the paper.} \\
% Department of Computer Science\\
% Cranberry-Lemon University\\
% Pittsburgh, PA 15213, USA \\
% \texttt{\{hippo,brain,jen\}@cs.cranberry-lemon.edu} \\
% \And
% Ji Q. Ren \& Yevgeny LeNet \\
% Department of Computational Neuroscience \\
% University of the Witwatersrand \\
% Joburg, South Africa \\
% \texttt{\{robot,net\}@wits.ac.za} \\
% \AND
% Coauthor \\
% Affiliation \\
% Address \\
% \texttt{email}
% }

% The \author macro works with any number of authors. There are two commands
% used to separate the names and addresses of multiple authors: \And and \AND.
%
% Using \And between authors leaves it to \LaTeX{} to determine where to break
% the lines. Using \AND forces a linebreak at that point. So, if \LaTeX{}
% puts 3 of 4 authors names on the first line, and the last on the second
% line, try using \AND instead of \And before the third author name.

% \iclrfinalcopy % Uncomment for camera-ready version, but NOT for submission.
\begin{document}

% More on Control and Interaction, not synthesizing
% First: synthesizing 发展的很快 -> HSI，Embodied AI & VR；
% Problems of previous methods 
% Ours 

% unified compare

\appendix
\input{sections/appendix}

\newpage

\bibliography{mainbib}
\bibliographystyle{iclr2024_conference}

\end{document}
